# Supplementary material for: Unlock the Power of Unlabeled Data in Language Driving Model
Source: arXiv:2503.10586 source file (2025-03-15)
Supplement: Supplementary file 1 [file appendix.tex]

\section*{APPENDIX}
